# Supplementary material for: Bridging the Gap Between Theory and Practice on Insertion-Intensive Database
Source: arXiv:2003.01064 source file (2020-03-02)
Supplement: Supplementary file 1 [file Appendix.tex]

\if 0
\begin{table*}
	\centering
	\begin{tabular}{|c|c|c|c|c|}\hline
		Algorithms	  &Amortized insertion cost 								     &Worst-case Insertion Cost	  &Query cost&Space required \\\hline 
	    B-tree \cite{BM72}&$O(\log_Bn)$&$O(\log_Bn)$&$O(\log_Bn)$	   &$O(\frac{n}{B})$\\\hline
		B$^\epsilon$-tree \cite{BF03} &$O(\frac{f\log_fB}{B}\log_B n)$&$O(\frac{f\log_fB}{B}\log_Bn)$ &$O(\log_fB\log_Bn)$&$O(\frac{n}{f})$\\\hline
		LSM-tree \cite{OCG+96} &$O(\frac{f\log_fB}{B}\log_B n)$&$O(\frac{n}{B})$&$O(\log_fB(\log_B n)^2)$&$O(\frac{n}{B})$\\\hline
		NB-tree (our paper)&$O(\frac{f\log_fB}{B}\log_Bn)$&$O(\frac{f\log_fB}{B}\log_Bn)$  &$O(\log_fs\log_B n)$ &$O(\frac{n}{B})$\\\hline
		
	\end{tabular}
	\caption{Summary of the theoretical results (performance in terms of cost)}
	\label{tab:summaryResults2}
\end{table*}

\begin{figure}
    \centering
    \begin{minipage}{.45\columnwidth}
	    \includegraphics[width=1\textwidth]{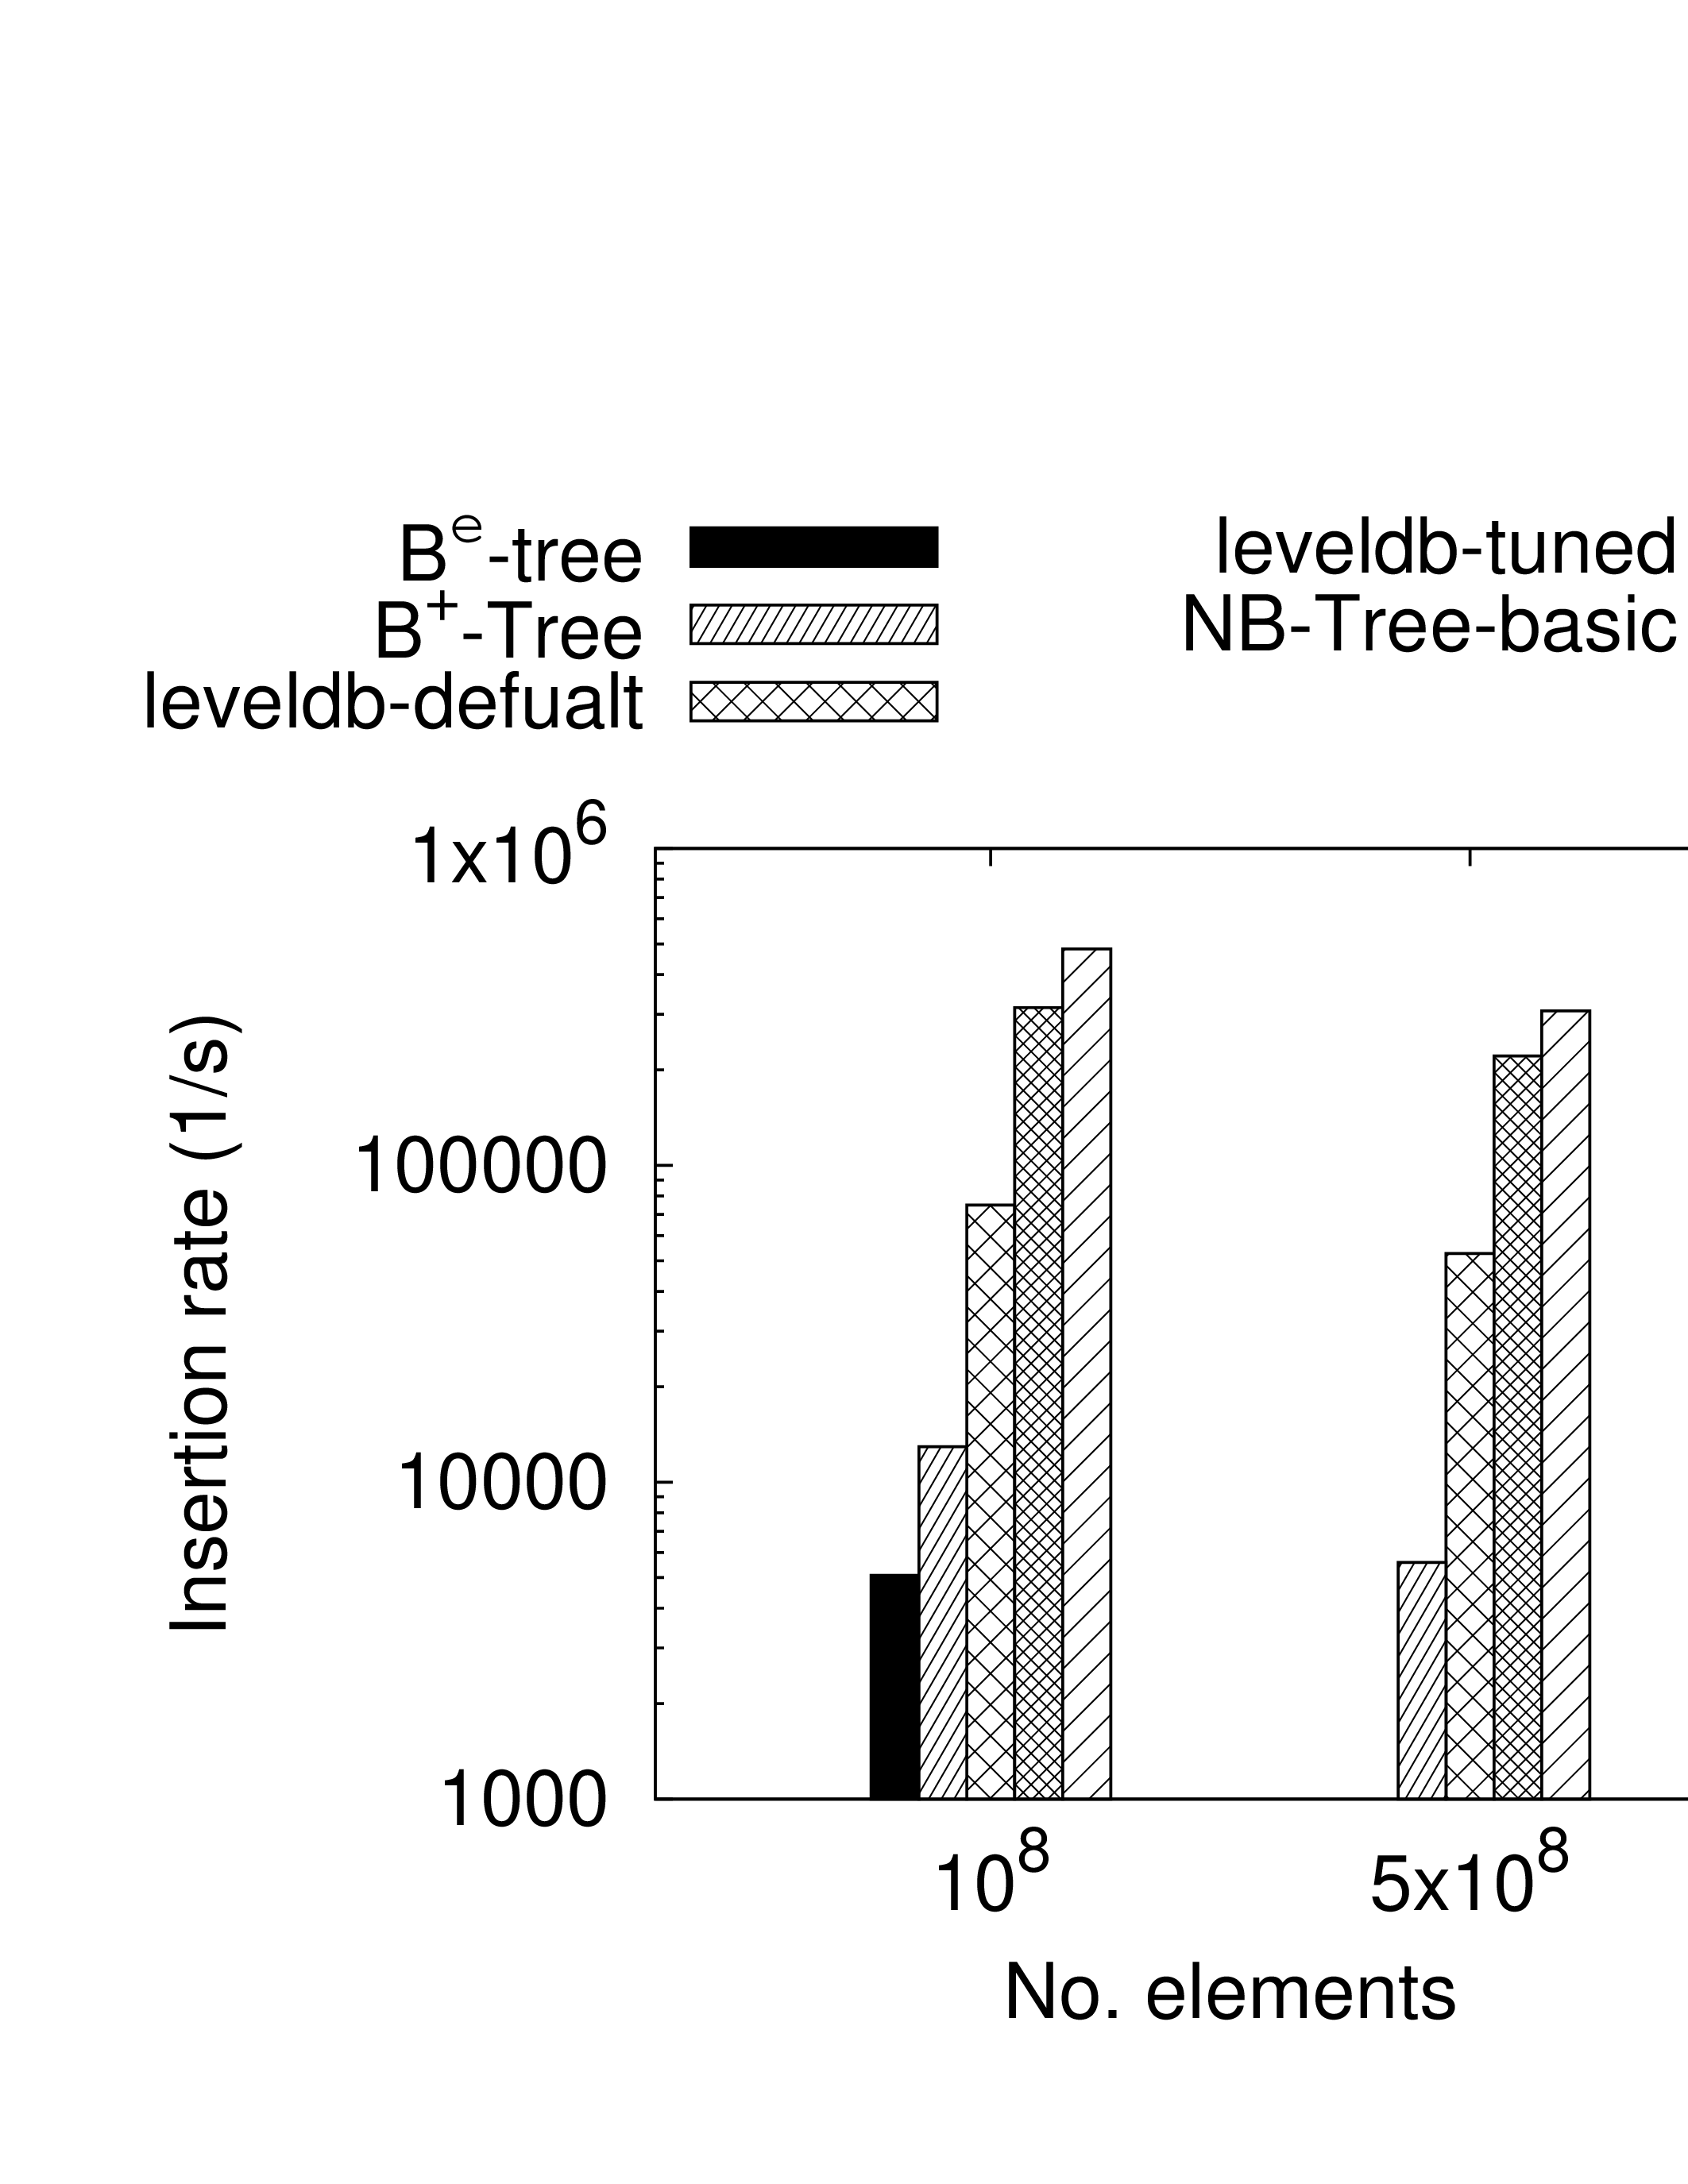}
        \vspace{-0.3cm}
        \caption{Performance on a Small Dataset}
      \label{fig:exp:small}
    \end{minipage}%
\hspace{0.3cm}
    \begin{minipage}{.45\columnwidth}
    	\includegraphics[width=1\textwidth]{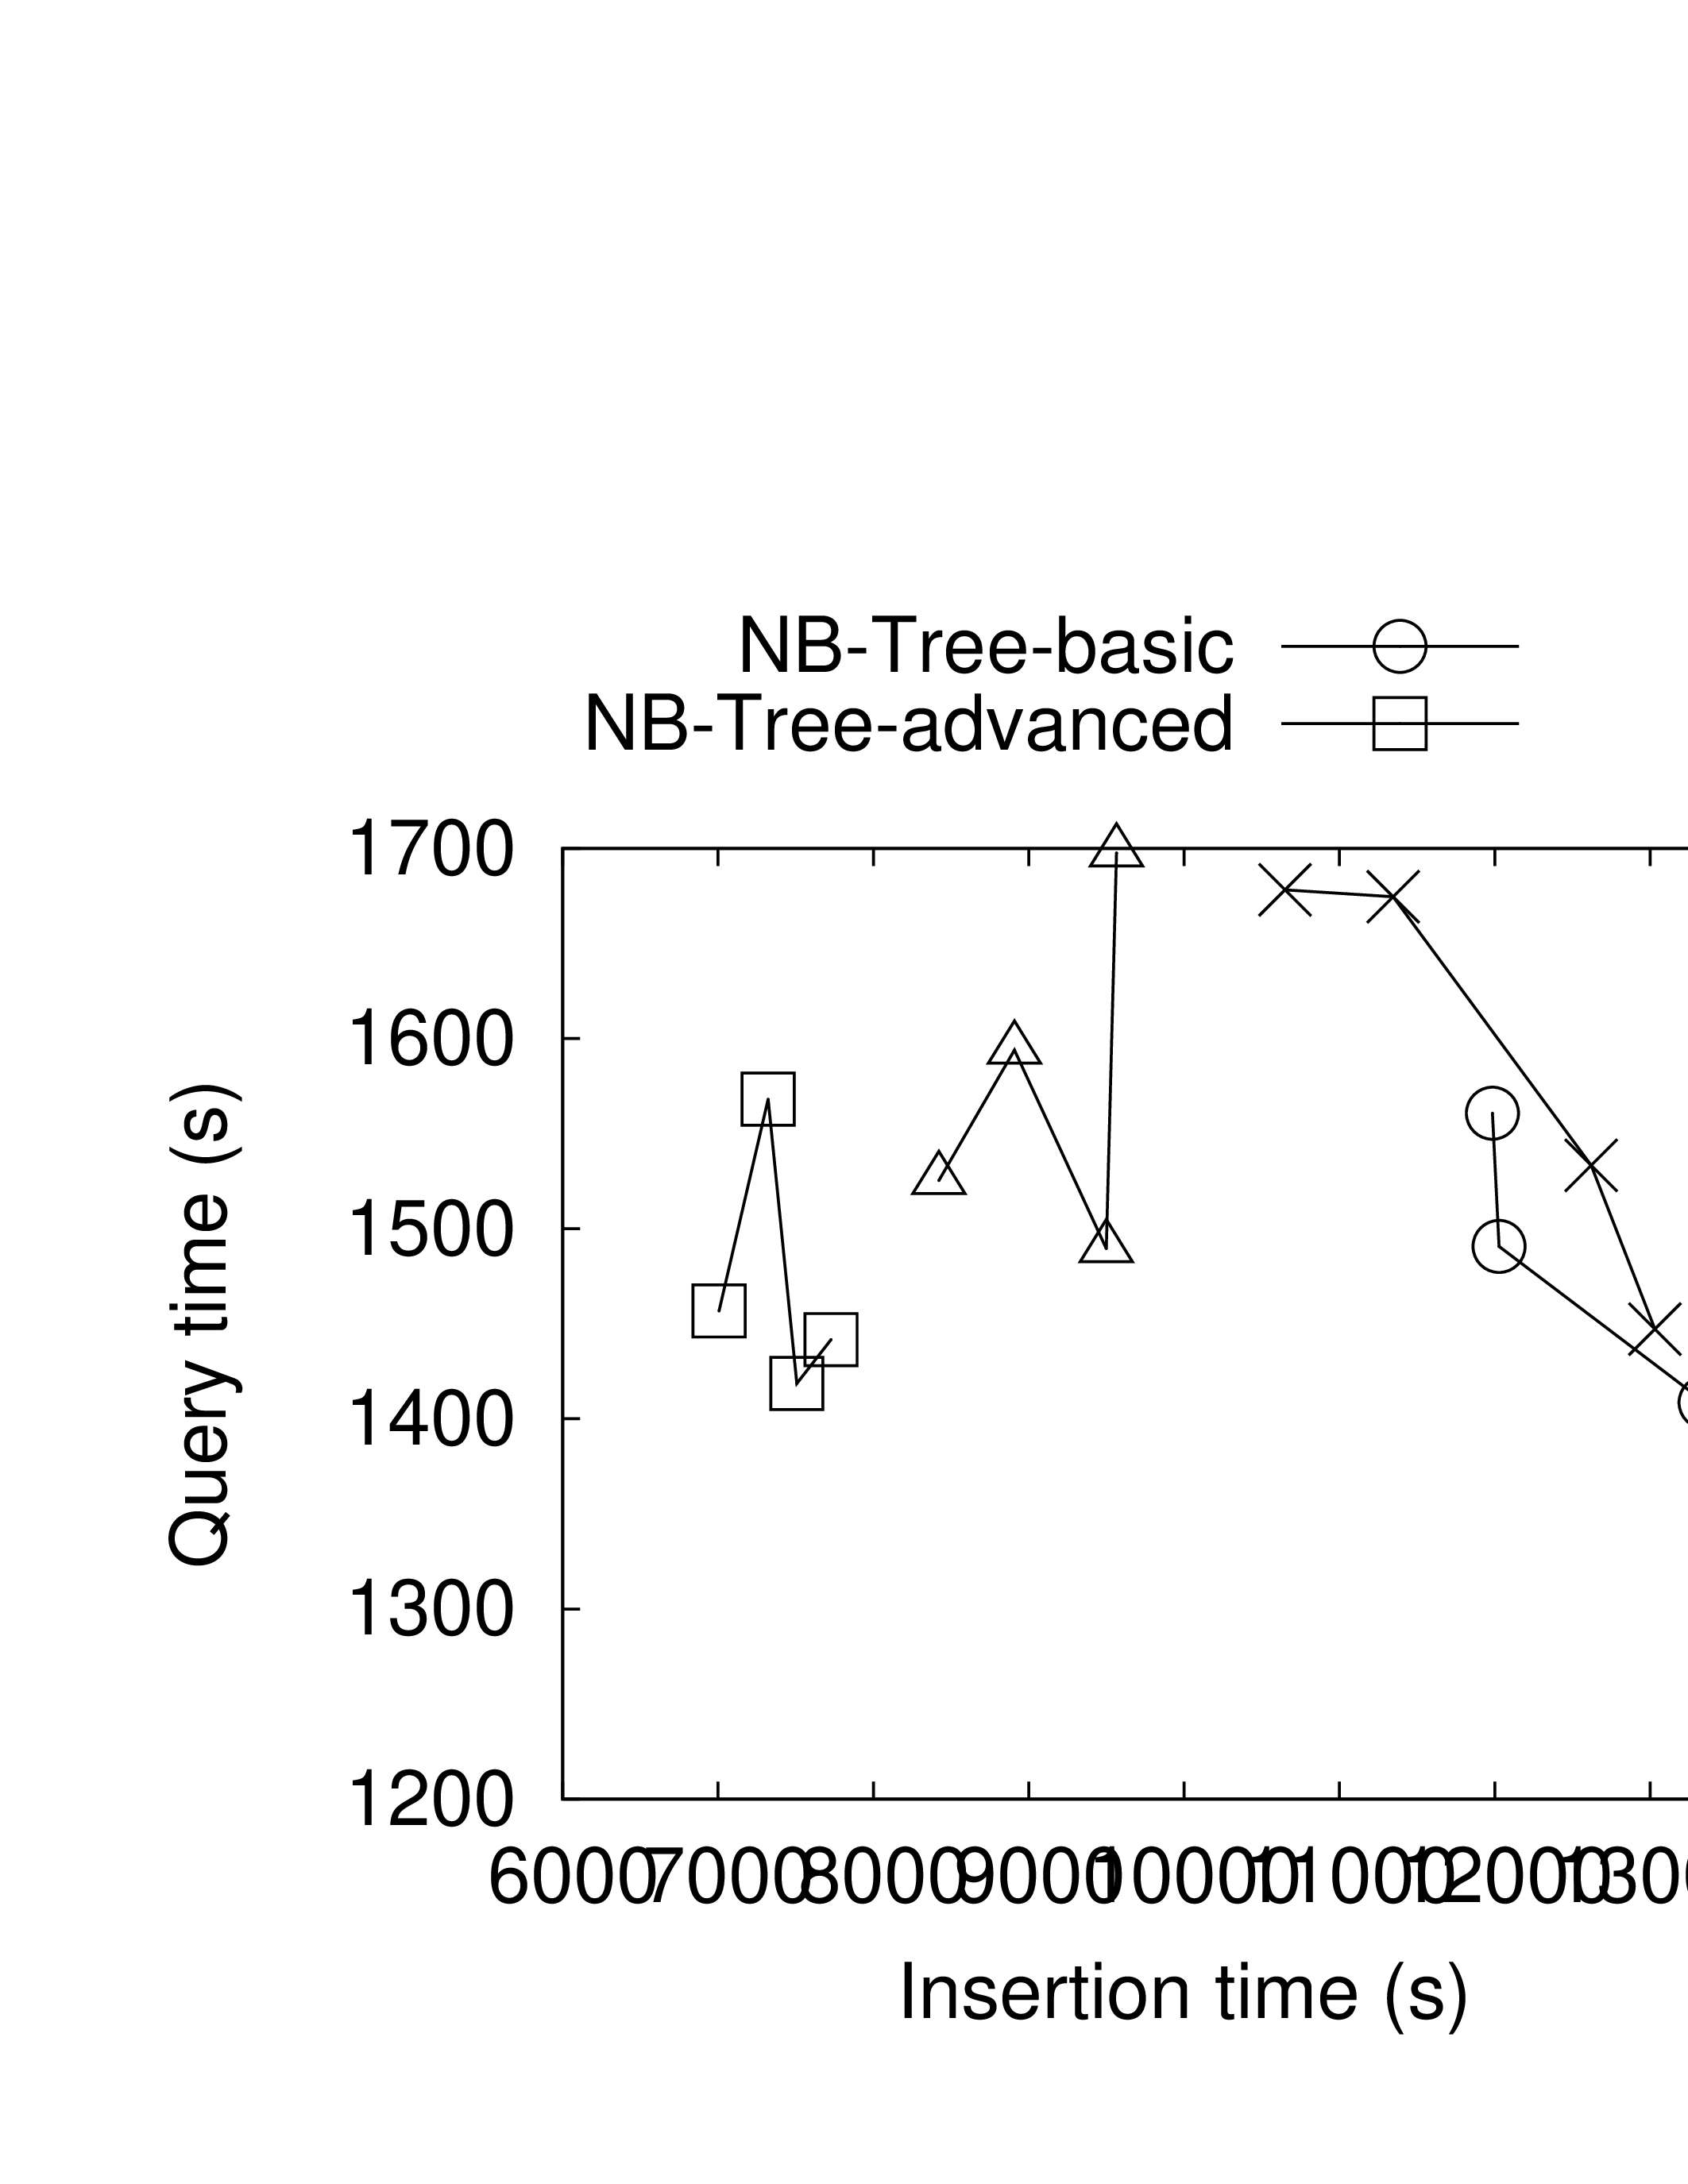}
\vspace{-0.3cm}
	    \caption{Query Time vs Insertion Time}
    	\label{fig:exp:QueryInsertion}   
    \end{minipage}%
\end{figure}

\begin{figure}
	\includegraphics[width=0.5\textwidth]{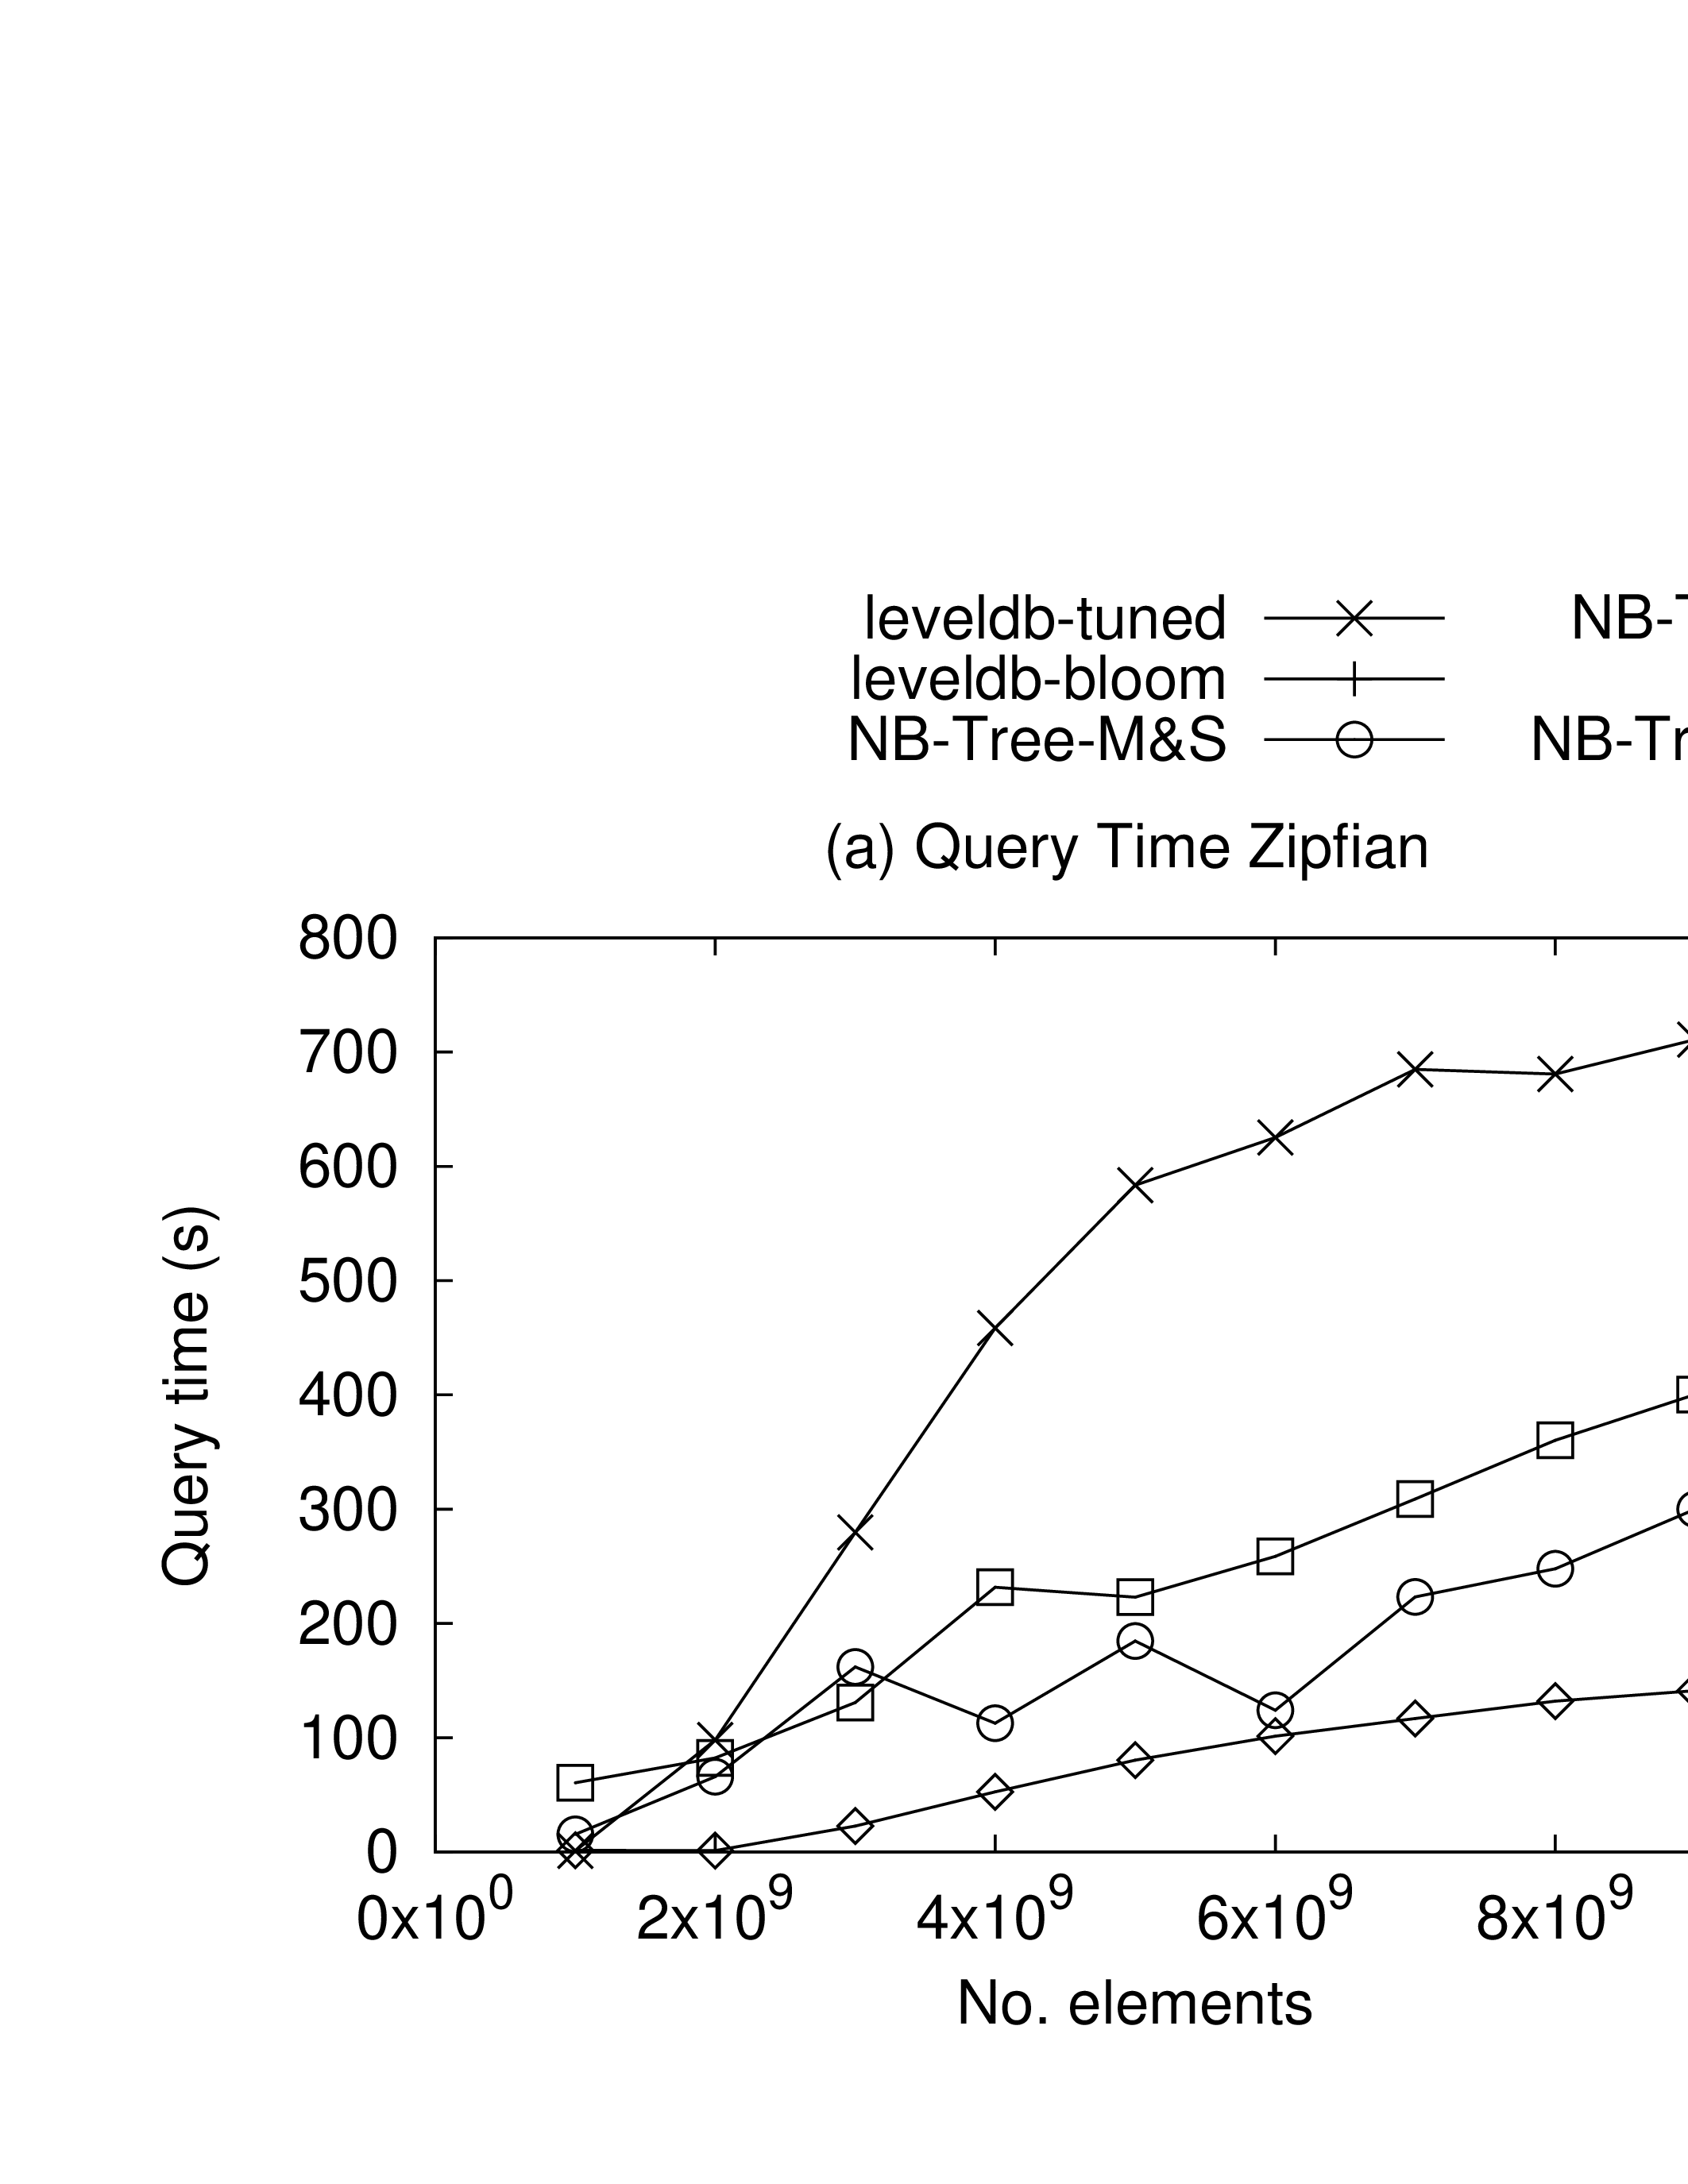}
	\caption{Zipfian Queries}
	\label{fig:exp:insertionDelayT1e5}
\end{figure}

\fi
